# Supplementary material for: Phase-Mapper: An AI Platform to Accelerate High Throughput Materials Discovery
Source: arXiv:1610.00689 source file (2016-10-07)
Supplement: Supplementary file 1 [file supplementary.tex]

\newpage

\section{Appendix}

\subsection{Proof of Theorem 3.1}
It is possible to show that the loss function is still non-decreasing when freezing complete parts of the matrices, and we will here briefly sketch the proof for the activation matrix, following closely CITE.

Denote the loss function when changing the activation matrix as $f(H)$. Due to linearity of the loss function with respect to the number of samples we assume that every $H^M$ is a column vector, if the loss function is non-increasing in this case it will be so in the general case by linearity. The proof that the update rules are non-increasing relies on a auxiliary function $G(H, H^\prime)$ that satisfies $G(H,H\prime) \geq f(H)$ and $G(H,H) = f(H)$, and it is easily proven that $f(H)$ is non-increasing under $H^{t+1} = argmin_H \quad G(H^t, H)$. For the generalized KL-divergence loss function the following auxiliary function is proposed in CITE, for which the above equations are satisfied.

\begin{align}
&\sum_i A_i log A_i - A_i + \sum_{i a m}  W_{ia}^{\downarrow m} H_a^m - \nonumber\\
&\sum_{i a m} A_i \frac{W_{i a}^{\downarrow m} H_a^{ \prime m}}{\sum_{b m} W_{ib}^{\downarrow m} H_b^{\prime m}} \bigg( log W_{ia}^{\downarrow m} H_a^m - log \frac{W_{i a}^{\downarrow m} H_a^{\prime m}}{\sum_b W_{ib}^{\downarrow m} H_b^{\prime m}} \bigg).
\end{align}

If we consider one or more components in the columns of $H$ and $H^\prime$ frozen to the same value we still get $G(H,H^\prime) = f(H)$. With $H$ frozen the equation $G(H,H^\prime) \geq f(H)$ is satisfied for all $H^\prime$, so we can additionally freeze some components of $H^\prime$ without changing that. When proving that the update rules results in non-increasing loss function we take $H^{t+1}=H^\prime$ such that it minimizes $G(H^\prime,H^t)$, chosing $H^{t+1}$ such that the gradient of $G$ is zero CITE. 

$$
\frac{\partial G(H^\prime, H^t)}{\partial H^{m}_a} = 0 = - \sum_i A_i \frac{W_{i a}^{\downarrow m} H^{m t}_a}{\sum_{b m} W_{ib}^{\downarrow m} H^{m t}_b} \frac{1}{H^{ m}_a} + \sum_i W_{ia}^{\downarrow m}
$$

$$
\implies H^{ m t+1}_a = \frac{H^{m t}_a}{\sum_i W_{ia}^{\downarrow m}} \sum_i A_i  \frac{W_{ia}^{\downarrow m}}{\sum_{bn} W_{ib}^{\downarrow n} H^{t n}_b}
$$

However, since the derivatives are taken component-wise the derivatives for the non-frozen components won't be changed by freezing some components. Thus we can use the update rules with some components frozen and still have the guarantee of non-increasing loss function. The update rules for keeping phases follows in the analogous same way since the two matrices play the same role and for the basis patterns the loss function is linear with respect to q-values.

\subsection{Proof of theorem \ref{thm:update_rule}}

\subsection{Proof of theorem \ref{thm:update_rule} and \ref{thm:update_rule_freeze}}

We will first sketch the proof for the loss function being non-increasing under the multiplicate update rules, following closely CITE[LEE seung]. Let us denote the loss function when changing the activation matrix as $f(H)$. Due to linearity of the loss function with respect to the number of samples we assume that every $H^M$ is a column vector, if the loss function is non-increasing in this case it will be so in the general case by linearity. The proof that the update rules are non-increasing relies on a auxilliary function $G(H, H^\prime)$ that satisfyes $G(H,H\prime) \geq f(H)$ and $G(H,H) = f(H)$, and it is easily seen that $f(H)$ is non-increasing under $H^{t+1} = argmin_H \quad G(H^t, H)$. For the generalized KL-divergence loss function the following auxialliary function is proposed in CITE, for which the above equations are satisfyed. For $G(H, H^\prime)$ we take

\begin{align}
&\sum_i A_i log A_i - A_i + \sum_{i a m}  W_{ia}^{\downarrow m} H_a^{\prime m} - \nonumber\\
&\sum_{i a m} A_i \frac{W_{i a}^{\downarrow m} H_a^{ \prime m}}{\sum_{b m} W_{ib}^{\downarrow m} H_b^{\prime m}} \bigg( log W_{ia}^{\downarrow m} H_a^m - log \frac{W_{i a}^{\downarrow m} H_a^{\prime m}}{\sum_b W_{ib}^{\downarrow m} H_b^{\prime m}} \bigg).
\end{align}

When proving that the update rules results in non-increasing lossfunction we take $H^{t+1}=H^\prime$ such that it minimizes $G(H^\prime,H^t)$, let us simply choses $H^{t+1}$ such that the gradient of $G$ is zero

$$
\frac{\partial G(H, H^t)}{\partial H^{m}_a} = 0 = - \sum_i A_i \frac{W_{i a}^{\downarrow m} H^{m t}_a}{\sum_{b m} W_{ib}^{\downarrow m} H^{m t}_b} \frac{1}{H^{ m}_a} + \sum_i W_{ia}^{\downarrow m}
$$

$$
\implies H^{ m t+1}_a = \frac{H^{m t}_a}{\sum_i W_{ia}^{\downarrow m}} \sum_i A_i  \frac{W_{ia}^{\downarrow m}}{\sum_{bn} W_{ib}^{\downarrow n} H^{t n}_b}
$$

%% If we see elements of $H^\prime$ as frozen then we don't take derivates with respect to them, and the derivates for the nonfrozen components wouldn't be changed by this. Thus since the update rules can be derived from setting the derivates to zero component-wise, we can use the update rules with some components frozen and still have guarantees of non-increasing loss function. The update rules for keeping phases follows in the analogous same way since the two matrices play the same role without sparsity, and for the basis patterns the loss function is linear with respect to q-values.

By equating $\sum_{bn} W_{ib}^{\downarrow n} H^{t n}_b = R_i$ we see that we obtain the update rules as per \ref{eq:kl_update2}.  Since the the above $H$ minimizes $G(H, H^T)$ which is an auxialliary function for our loss function, it is guaranteed to be non-increasing. Deriving the update rules, and showing that the loss function is non-increasing under them, is done analogously for the $W$ matrices.

%If we see elements of $H^\prime$ as frozen then we don't take derivates with respect to them, and the derivates for the nonfrozen components wouldn't be changed by this. Thus since the update rules can be derived from setting the derivates to zero component-wise, we can use the update rules with some components frozen and still have guarantees of non-increasing loss function. The update rules for keeping phases follows in the analogous same way since the two matrices play the same role without sparsity, and for the basis patterns the loss function is linear with respect to q-values.

It is possible to show that the loss function is still non-decreasing when freezing complete parts of the matrices, and we will here outline the proof for the activation matrix, as before we take $H$ to be a column matrix which is sufficient by linearity of the loss function. If we consider one or more components in the columns of $H$ and $H^\prime$ frozen to the same value we still get $G(H,H^\prime) = f(H)$. With $H$ frozen the equation $G(H,H^\prime) \geq f(H)$ is satisfied for all $H^\prime$, so we can additionally freeze some components of $H^\prime$ without changing that. However, since the derivatives are taken component-wise the derivatives for the non-frozen components won't be changed by freezing some components. Thus we can use the update rules with some components frozen and still have the guarantee of non-increasing loss function. The update rules for keeping phases follows in the analogous same way since the two matrices play the same role and for the basis patterns the loss function is linear with respect to q-values.
